# Supplementary material for: Systematic Mutation-based Evaluation of the Soundness of Security-focused Android Static Analysis Techniques
Source: arXiv:2102.06829 source file (2021-07-17)
Supplement: Supplementary file 1 [file appendix_tools.tex]

\section{Lessons learned from exploring other static analysis tools
\label{appendix_tools}

To understand the applicability of \tool{}, we run several static analysis tools, namely HornDroid~\cite{cgm16}, AmanDroid~\cite{wror14}, and FlowDroid~\cite{arf+14}, against the \counttotalmutantapps{} mutated apps we generated in Section~\ref{sec:executing_tools}.
    This is done to determine the compatibility of these tools with the mutated apps, and whether these tools can detect the inserted leaks.
    Then, we perform frequency analysis to determine whether the tools are able to detect all the inserted leaks.
    Next, for each tool, we use number of undetected leaks at a per-class per-method basis to prioritize manual analysis of leaks inserted at classes and methods.
    Finally, we extract those leaks and prepare minimal APKs, each containing only one leak contained within the essence of structure from the mutated apps.
    We use these minimal APKs for further analysis of these tools.

To conduct this study, we created an environment in a virtual server with 32GB of RAM and 8 cores in Intel Haswell Processor,
with Ubuntu 64 bit 16.04.6 LT. We installed and run each of the static analysis tools according to the instructions provided with their code-bases. We installed the different required versions of Android platform to make sure that our used tools were properly configured. During the execution of the tools, we set a cutoff time of 36 hours per mutated app analysis.
\KEVIN{What were these tools being run against here?? A single application, all generated executable mutants, this must be specified.}
If we do not get result for a mutated app within the cut-off time, we classify the app as incompatible with the tool and proceed to the next app. We use the default configuration parameters of each tool, and modify the source or sink definition file as necessary to allow for the detection of leaks in our mutated applications. Our findings, along with brief reasons of using the tools can be summarized as follows:

\myparagraph{FlowDroid}{ \add{FlowDroid is a tool  introduced by Artz et al.~\cite{arf+14} as a data leak detection tool for Android in 2014. It modeled the Android life-cycle to handle callbacks invoked by the Android Framework to perform information flow analysis and data leak detection. Furthermore, it applied context, flow, field, and object-sensitivity to reduce the number of false positive sensitive data leaks the tool detects.} \add{This tool has been continuously maintained, with the latest release being FlowDroid v\(2.7.1\), which was made available on January 21, 2019. It has been cited for 700+ times, which further motivated us to use this tool. The current oldest available release is FlowDroid v\(2.5.1\). Our study spanned over an year and only FlowDroid v\(2.0\) was available during when we initially selected apps 01-07 as base apps for mutation. We generated  21 mutated apps using the earlier version of \tool{} for base app 01-07 and analyzed them using FlowDroid v\(2.0\). We observed that it was compatible with all 21 mutated apps, detecting 48.7\% executable leaks.}
\KEVIN{Give numbers here, was it incompatible with any apps \textbf{why}?}}\AMIT{Done}

\myparagraph{HornDroid}{\add{HornDroid was introduced by  Calzavara et al.~\cite{cgm16} as the first static analysis tool in Android with a formal proof of soundness. HornDroid abstracts Android applications as a set of Horn clauses to formulate security properties, which can then be processed by other Satisfiability Modulo Theories (SMT) solvers. Moreover, we chose HornDroid especially because it works by using a formally verified  model of activity lifecycle. Moreover, the authors of HornDroid state that, \textit{"In order to support a sound analysis of fragments, HornDroid over-approximates their life-cycle by executing all the fragments along with the containing activity in a flow-insensitive way".}
Additionally, HornDroid employs flow-sensitive analysis, and for achieving soundness it uses flow-insensitive analysis for static fields. HornDroid authors mentioned that they performed experiments on a server with 64 multi-thread cores and 758 Gb of memory, although they reported that the most memory utilization was around 10 Gb. Moreover, all the Android applications they evaluated their approach on were of Android API version 19. Our environment setup matches this. Even though HornDroid did not give us any conclusive result for 4 out of 31 mutated apps created from base apps 08-15 either due to memory insufficiency error, or execution crashes; we still included it within our shortlist of in-depth analysis due to its formally verified model for soundness.}\KEVIN{Same thing, give numbers here, How many apps was it incompatible with and \textbf{why}?}}\AMIT{Done}

\myparagraph{AmanDroid}{\add{Using a combination of context-sensitive and flow-sensitive inter-component data flow graph (IDFG), and data dependence graph (DDG); Wei et al.~\cite{wror14} proposed AmanDroid could be used for different types of security analysis, including information leak from a sensitive source to a critical sink. Presently known as Argus, AmanDroid is being actively maintained and has over 200+ citations. There are several publicly available versions of this tool, with the latest two being v{$3.1.2$} and v{$3.2.0$}. As version v{$3.2.0$} is officially stated to be ``\textit{pre-release for the next major release}'', we used v\(3.1.2\) for our feasibility study. We found that it successfully completed analysis for all 31 mutated apps created from the base app 07-15; detecting 74\% of the inserted leaks.}\KEVIN{Give numbers here, How many apps was it incompatible with and \textbf{why}?}}\AMIT{Done}
\add{
It should be mentioned that we intentionally used mutated apps from base apps 01-07 and 08-15 separately for the static analysis tools. There are two reasons behind this. First, applying different set of apps allow us observe whether \tool{} can be used to find \soundiness{} issues without depending too much on the base apps being used.  To elaborate, we use the first set of mutated apps to analyze whether there are any \soundiness{} issues or flaws in FlowDroid v\(2.0\). If any such flaws are found, propagation study is done to understand whether other tools additionally have similar \soundiness{} issues. Next, we use the second set of mutated apps to analyze Argus v\(3.1.2\) and HornDroid to find \soundiness{} issues, and do a similar propagation study. This way, we can observe whether using a different set of apps can yield previously unseen \soundiness{} issues across tools.

Second and more importantly, our intuition is that \textit{benchmarks for evolving platforms such as Android should evolve with time}.
%got it from insight 7
Static analysis tools often become inapplicable or unusable due to one of several confounding, external factors. In particular, we identify three major factors that may hinder the use and applicability of static analysis tools as well as static benchmarks: (i) The evolution of Android OS components, (ii) the evolution of application platforms, and (iii) the evolution of the Android SDK. To the first point, components within the Android OS are continuously evolving, which in turn changes how apps interact or are managed by the host operating system. Moreover, these changes are often introduced in layers to ensure backward compatibility, thus offering a consistent experience across the platform segments. Static analysis tools that were designed to analyze an older set of Android OS components, may not necessarily be applicable to newer components. For the second factor, the components that make up apps are changing as well, either trough the introduction of new widgets or via changes to existing widgets that affect how users interact with them. A dataflow analysis tool that expects a certain set of app widgets or behaviors, may not necessarily function properly on updated widgets or behaviors. Finally, the Android Standard Development Kit (SDK) and its associated tools are frequently being changed as well. For example, the Eclipse Android Development Tool (ADT) plug-in was the official tool for creating Android Apps before 2015. Thus, many components of the SDK were tightly coupled to Eclipse. However, after 2015 the support and development of Eclipse ADT were officially ended~\cite{android-adt-obsolete} and Android Studio IDE was introduced. Thus static analysis tools that were meant to interface with Eclipse may no longer function properly with modern Android development tool-chains. Therefore, relying on a static benchmark that does not evolve with the platform can only give a false sense of soundness, while in actuality, it is merely \soundiness{}. We further discuss some other lessons learned related to software evolution and aging while exploring other existing static analysis tools in the Appendix \ref{appendix_tools}.
}

\myparagraph{BlueSeal}{\add{Shen et Al.\cite{svt+14} proposed that \textit{Flow  Permissions} should be used in addition to the existing Android permissions approach to give better control of information control to users. As part of this approach, they further created a static analysis engine called BlueSeal for offline app analysis.} \add{We went through the official repository of BlueSeal and found that as of August 26, 2019, the only available release was declared to be temporary 5 years ago, and \textit{``The full-published version will be available soon.''}. }}

\myparagraph{IccTA}{\add{IccTA is a static taint analyzer introduced by Li et  al.~\cite{lbb+15}, which focused on leaks in inter-component communication. } \add{Historically, IccTA was built on top of FlowDroid. However, its last update was in 2016 and there is no indication of it being compatible with FlowDroid's latest releases. Moreover, it is mentioned in the release of FlowDroid 2.5.1 that \textit{``IccTA is already onboard since version 2.0''}, thus allowing us to assume that later releases of FlowDroid already covers all functionalities offered by IccTA. }}

\myparagraph{DroidSafe}{\add{Gordon et al.~\cite{gkp+15} proposed that  DroidSafe, a static information flow analysis tool, can be used to detect information leaks as it creates a model of Android Runtime with static analysis design decisions.} \add{Based on the description in the official repository of DroidSafe, it is expected to perform well when certain restrictions are met, including but not limited to only using apps which do not require Google Play, apps which use a limited set of Android API classes, and apps which are specifically built for Android 4.4.1 released in December 2013, and contains at most 50K Lines of Codes including libraries. Our observation is that real-life apps often are not restricted by these conditions.}

\myparagraph{DidFail}{\add{Droid Intent Data Flow Analysis for Information  Leakage ({\sc Didfail}) by Klieber et al.~\cite{kfb+14} builds on the works of FlowDroid~\cite{arf+14}, Soot~\cite{vcg+99} and Epicc(Effective Inter-Component Communication Mapping in Android)~\cite{octeauEffectiveIntercomponentCommunication2013}. For taint analysis, it uses FlowDroid for inter-component and Epicc for intra-component analysis.}
